# Supplementary material for: Binary Black Holes in Modified Gravity
Source: arXiv:2308.12037 source file (2023-08-23)
Supplement: Supplementary file 1 [file adm_mass_bubbles.tex]

\section{ADM mass of scalar field bubbles}

In section \ref{subsec:paper1:initial_data}, the total energy density was calculated as $\rho_0 = \int_{\mathcal{R}^3}\r\, d^3x$, which assumes a Minkowski flat background, when in reality the formula is $\rho_0 = \int_{\mathcal{R}^3}\r \sqrt{\g}\, d^3x$, with $\sqrt{\g}=\chi^{-\tfrac{3}{2}}$. I don't know why, but by solving the constraints as detailed in this section, the correct energy density is $\r_{final}=\frac{\r_0}{\chi_{r=0}}$. I don't know why this happened to be true. Furthermore, I realised that one could parametrise the solution of $\chi$ of the constraints at $r=0$ as (within a reasonable range of the parameters, and only when $g_2$ and $g_3$ are suitably small in comparison to GR) $\chi_{r=0}=1-\frac{A^2r_0}{2\w}$.

It is interesting to explore 
\todo{Show how we fitted $\chi_{r=0}=1-\frac{A^2r_0}{2\w}$}
